# Supplementary material for: Retrieval of aerosol properties from in situ, multi-angle light scattering measurements using invertible neural networks
Source: arXiv:2111.07960 source file (2021-11-15)
Supplement: Supplementary file 1 [file additional_info.tex]

\documentclass[11pt,a4paper]{article}
\usepackage{hyperref}
\setlength\parindent{0pt}
\begin{document}
\textbf{CRediT author statement:}

\url{https://www.elsevier.com/authors/policies-and-guidelines/credit-author-statement}

Romana Boiger: Writing - Original Draft, Conceptualization, Software, Validation, Visualization, Formal analysis, Funding acquisition 

Rob L. Modini: Writing - Original Draft, Conceptualization, Data curation

Alireza Mallemi: Investigation, Resources, Data curation, Writing - Reviewing and Editing

David Degen: Software, Validation, Visualization, Writing - Reviewing and Editing

Martin Gysel-Beer: Supervision, Writing - Reviewing and Editing, Funding acquisition 

Andreas Adelmann: Supervision, Writing - Reviewing and Editing

\textbf{Highlights}
https://www.overleaf.com/project/60992c56b10c8e32ca4da849
https://www.overleaf.com/project/60992c56b10c8e32ca4da849

Not part of editorial consideration and aren't required until the final files stage

\url{https://www.elsevier.com/authors/tools-and-resources/highlights}

\begin{itemize}
    \item Forward and inverse surrogate models for simulating aerosol measurements and retrieving aerosol properties from measurement data.
    \item The aerosol retrieval method is demonstrated to be both fast and accurate. 
    \item Extensive case study including measurement errors shows the practical applicability.
\end{itemize}

\textbf{Short statement of novelty}

(We request that you include a short statement of novelty to your submission. This statement should describe what your research is adding to the existing literature and should be limited to 120 words.)

The present study proposes a new method to retrieve aerosol properties from in situ light scattering data based on invertible neural networks (INNs). The proposed method is novel for two main reasons. Firstly, it represents the first application of machine learning to simulated measurement data from a new type of instrument – a laser-imaging type polar nephelometer. The results show that the method is both fast and accurate relative to current state-of-the-art retrieval methods (e.g. look-up tables, physics-based inversion models). Secondly, the method demonstrates a new way of utilizing the unique architecture of INNs. Specifically, the algorithm is not only able to accurately retrieve aerosol properties from measurement data, but also to simulate measurement data given aerosol properties.

\textbf{Cover letter}

Dear Editors, 

we are submitting our manuscript \textbf{Retrieval of aerosol properties from in situ, multi-angle light scattering measurements using invertible neural networks} to be considered as an article for publication in the Journal of Computational Physics.

Aerosols play an important role for the development of Earth's climate and have a huge impact on public health. To better understand their influence, in-situ light scattering measurements can provide substantial information on aerosol properties. So, retrieving this information from measurement data is an important task. The current state of the art retrieval methods suffer from either speed or accuracy limitations that are becoming increasingly restrictive as instrumentation complexity increases and new measurement applications arise.  

Our contribution helps to resolve this issue by introducing an inverse model based on invertible neural networks. We demonstrate that this model is both fast and accurate under both ideal simulated measurement conditions, as well as real world conditions involving noisy data and imperfect measurement data. The high accuracy, the little computational effort and the fast evaluation of the inverse model pave the way for online or near-real-time aerosol retrieval calculations from measurements obtained with new and potentially miniaturized sensors.

In addition, the method we propose accomplishes a second task, it provides a surrogate model that can predict measurement data from aerosol properties. Once the model is trained, the computational effort is negligible and hence it can replace standard physics based models when very fast computations are required.

None of the material has been published or is under consideration elsewhere.
We hope our contribution will be considered for in-depth review and look forward to hearing from you.

Thank you for your attention in this matter.

Sincerely, 

Dr. Andreas Adelmann

Head of the Laboratory for Scientific Computing and Modelling

\end{document}
